# Supplementary material for: Adversarial NLI: A New Benchmark for Natural Language Understanding
Source: arXiv:1910.14599 source file (2020-05-06)
Supplement: Supplementary file 1 [file appendix.tex]

%
% File acl2020.tex
%
%% Based on the style files for ACL 2020, which were
%% Based on the style files for ACL 2018, NAACL 2018/19, which were
%% Based on the style files for ACL-2015, with some improvements
%%  taken from the NAACL-2016 style
%% Based on the style files for ACL-2014, which were, in turn,
%% based on ACL-2013, ACL-2012, ACL-2011, ACL-2010, ACL-IJCNLP-2009,
%% EACL-2009, IJCNLP-2008...
%% Based on the style files for EACL 2006 by 
%%e.agirre@ehu.es or Sergi.Balari@uab.es
%% and that of ACL 08 by Joakim Nivre and Noah Smith

\documentclass[11pt,a4paper]{article}
\usepackage[hyperref]{acl2020}
\usepackage{times}
\usepackage{latexsym}
\usepackage{amssymb}
\usepackage{amsmath}
\usepackage{booktabs}
\usepackage{multirow}
\usepackage{multicol}
\usepackage{tipa} % for pretty french accents

%% put false in the brackets to shut of the notes
\usepackage[]{todonotes}

\newcommand*\iftodonotes{\if@todonotes@disabled\expandafter\@secondoftwo\else\expandafter\@firstoftwo\fi}

% This is not strictly necessary, and may be commented out,
% but it will improve the layout of the manuscript,
% and will typically save some space.
\usepackage{microtype}

%\aclfinalcopy % Uncomment this line for the final submission
 %  Enter the acl Paper ID here

\title{Adversarial NLI: Supplementary Material}

%\author{Yixin Nie$^*$, Adina Williams$^\dagger$, Emily Dinan$^\dagger$, Mohit Bansal$^*$, Jason Weston$^\dagger$, Douwe Kiela$^\dagger$\\
%  $^*$UNC Chapel Hill\\$^\dagger$Facebook AI Research\\}

\date{}

\begin{document}
\maketitle

\renewcommand\thesection{\Alph{section}}
\input{supplementary/realappendix.tex}

\newpage

\bibliography{acl2020}
\bibliographystyle{acl_natbib}

\end{document}
